# Supplementary material for: Quantum limits to the energy resolution of magnetic field sensors
Source: arXiv:1905.00618 source file (2020-01-06)
Supplement: Supplementary file 1 [file SI.tex]

This file exist only to run BibTeX from.
